# Supplementary material for: Exact and Perturbed Friedmann-Lemaitre Cosmologies
Source: arXiv:0709.3863 source file (2007-09-25)
Supplement: Supplementary file 1 [file Appendix-FLExistenceUniqueness.tex]

\chapter{Existence-Uniqueness for the Friedmann Equation} \label{chap:FLexistenceuniqueness}

In this appendix, we will prove an important result required to ensure existence-uniqueness of solutions to the Friedmann DE (\ref{eq:FLDimlessLDE}), given by
\begin{equation} \label{FLEUeq:FLDimlessLDE}
\left( \frac{dL}{dT} \right)^2 = \sum_{i=1}^{n} m_i L^{-3 \gamma_i + 2} - K,
\end{equation} for any choice of parameters $m_i > 0$, $i = 1, \ldots, n-1$ and subject to the conditions
\begin{equation}
L(0) = 0, \quad \mbox{and} \quad \frac{dL}{dT}(0) > 0,
\end{equation}  We note that a similar approach can be used to show existence-uniqueness of the Friedmann DE, written using observational parameters (\ref{eq:FLObservationalDE}).

We can rewrite (\ref{FLEUeq:FLDimlessLDE}) as
\begin{equation}
\left( \frac{dL}{dT} \right)^2 = L^{-(3 \gamma_1 - 2)} \left[ \sum_{i = 1}^{n} m_i L^{3 (\gamma_1 - \gamma_i)} - K L^{3 \gamma_1 - 2} \right].
\end{equation}  Since $\gamma_1 > \gamma_2 > \cdots > \gamma_n$ and $\gamma_1 > \tfrac{2}{3}$, this DE is of the form
\begin{equation} \label{FLEUeq:FLDimlessLDE2}
\left( \frac{dL}{dT} \right)^2 = L^{- (3 \gamma_1 - 2)} F(L),
\end{equation} with
\begin{equation}
F(0) = m_1 > 0.
\end{equation}  Assuming $\frac{dL}{dT} > 0$, which clearly holds in any expanding domain, we can rewrite (\ref{FLEUeq:FLDimlessLDE2}) as
\begin{equation} \label{FLEUeq:FLDimlessLDE3}
\frac{dT}{dL} = \frac{L^{\frac{1}{2} (3 \gamma_1 - 2)}}{F(L)^{1/2}}, \qquad L \geq 0.
\end{equation}  The general solution to (\ref{FLEUeq:FLDimlessLDE3}) is then, for all $m_i > 0$,
\begin{equation}
T = G(L) + C,
\end{equation} where $G(L)$ is the antiderivative of the RHS of (\ref{FLEUeq:FLDimlessLDE3}).  The requirement that $T = 0$ when $L = 0$ fixes $C$, and hence gives a unique solution.
